# Supplementary material for: Deciphering the Definition of Adversarial Robustness for post-hoc OOD Detectors
Source: arXiv:2406.15104 source file (2025-01-29)
Supplement: Supplementary file 1 [file supplementary.tex]

\section{OOD Definition per Method} \label{app:definition}

This section extends the \cref{sec:definition}.
In \cref{tab:def}, we compare the chosen ID and OOD datasets of each OOD detector. 
In this comparison, we pick those experiments with largest dimensioned available datasets.
Furthermore, we extend this comparison by appending the adversarial robust OOD detectors from the related work in \cref{sec:adv_defenses}. 
It can be observed that the more recent post-hoc detectors tend to have ImageNet-1K as standard ID datasets. 
In contrast, the adversarial robust OOD detectors are benchmarked more likely on the smaller and less complex CIFAR-10 dataset. \\

\noindent Following attacks, models, and datasets are used to heuristically evaluate OOD samples (more details in \cref{tab:def}): 

\noindent \textbf{Attacks}: FGSM \cite{goodfellow2014explaining}, PGD \cite{madry2017towards}

\noindent \textbf{Model Architectures}: 
\begin{itemize}[nosep]
\item ResNet-18/ResNet-50 \cite{he2016deep}, ResNetv2-101 \cite{he2016identity}, ResNet-50-D \cite{touvron2019fixing}, TResNet-M \cite{ridnik2021tresnet}, WideResNet \cite{zagoruyko2016wide}
\item BiT \cite{kolesnikov2020big}, VIT-B-16 \cite{dosovitskiy2020image}, ViT \cite{touvron2021training}, DeiT \cite{touvron2021training}, Swin-T \cite{liu2021swin} 
\item DenseNet-121 \& DenseNet-101 \cite{huang2017densely}
\item MobileNet \cite{howard2017mobilenets}, MobileNetV2 \cite{sandler2018mobilenetv2}
\item RegNet \& RegNetX4.0 \cite{radosavovic2020designing}
\item RepVGG \cite{ding2021repvgg}
\item Mixer-B-16 \cite{tolstikhin2021mlp}
\item CLIP \cite{radford2021learning}
\end{itemize}

\noindent \textbf{Datasets}: CIFAR-10/CIFAR100 \cite{krizhevsky2009cifar}, BDD-Anomaly  \cite{hendrycks2019scaling}, DeepDrive \cite{wu2022decentralized}  ImageNet-1K \cite{deng2009imagenet}, ImageNet-21K \cite{ridnik2021imagenet}, ImageNet-O \cite{hendrycks2019benchmarking}, iNaturalist \cite{van2018inaturalist},  ISUN \cite{quattoni2009recognizing}, GSTRB \cite{stallkamp2012man}, LSUN \cite{yu2015lsun}, NINCO \cite{bitterwolf2023or},  OpenImage-O \cite{wang2022vim},  Pascal-VOC \cite{hoiem2009pascal}, Places \cite{zhou2017places}, Textures \cite{cimpoi2014describing}, TinyImageNet \cite{le2015tiny}, Species \cite{van2015building},  StreetHazards \cite{hendrycks2019scaling}, SSB-hard \cite{vaze2021open}, SVHN \cite{netzer2011reading}, SUN \cite{xiao2010sun}. \\

\begin{table*}[tb]
\centering
\caption{\small
Overview of ID and OOD definition from several OOD detectors.
The detectors are divided into the following categories \cite{zhang2023openood}:
 \colorbox[HTML]{FED8E5}{Classifiction-based}, \colorbox[HTML]{CFE7FF}{Density-based}, \colorbox[HTML]{F3D5B0}{Distance-based}. We also mark:  \colorbox[HTML]{70AD47}{Supervised and Adversarial Robust}.
} \label{tab:def}
\resizebox{!}{0.48\textheight}{
\begin{tabular}{p{0.1\textwidth}|p{0.2\textwidth}p{0.3\textwidth}p{0.3\textwidth}}
    \toprule[1pt]
    \hline
    \textbf{Methods} &
      \textbf{ID} &
      \textbf{OOD} &
      \textbf{Model Architectures} \\ \hline     \hline   
    \multicolumn{4}{c}{PostHoc Methods} \\ \hline    
    % OpenOOD \cite{zhang2023openood} &
    %   ImageNet-1K &
    %   Near-OOD: SSB-hard, NINCO; Far-OOD: iNaturalist, Textures, OpenImage-O; Covariate-Shifted ID: ImgeNet-C, ImageNet-R, ImageNet-v2 &
    %   ResNet-50, Swin-T,   VIT-B-16 \\ \hline
    \rowcolor[HTML]{FED8E5} 
    SCALE \cite{xu2023scaling} &
      ImageNet-1K &
      Near-OOD: NINCO, SSB-hard; Far-OOD: iNaturalist,  OpenImage-O, Textures
      & ResNet-50 \\
    \rowcolor[HTML]{FED8E5} 
    NNGuide \cite{park2023nearest} &
      ImageNet-1K &
      Near-OOD: iNaturalist, OpenImage-O; Far-OOD: Textures; Overlapping: SUN and Places &
      MobileNet, RegNet, ResNet-50, ViT \\
    \rowcolor[HTML]{FED8E5} 
    GEN \cite{liu2023gen} &
      ImageNet-1K &
      ImageNet-O, iNaturalist, OpenImage-O, Texture,  &
      BiT, DeiT, RepVGG, ResNet-50, ResNet-50-D, Swin-T, ViT \\
    \rowcolor[HTML]{FED8E5} 
    ASH \cite{djurisic2022extremely} &
      ImageNet-1K &
      iNaturalist, Places, SUN, Textures &
      MobileNetV2, ResNet-50 \\
    \rowcolor[HTML]{CFE7FF} 
    DICE \cite{sun2022dice} &
      ImageNet-1K &
        iNaturalist, Places, SUN, Textures &
      DenseNet-101 \\
    \rowcolor[HTML]{FED8E5} 
    KNN \cite{sun2022out} &
      ImageNet-1K &
        iNaturalist, Places, SUN, Textures &
      ResNet-50 \\
    \rowcolor[HTML]{FED8E5} 
    VIM \cite{wang2022vim} &
      ImageNet-1K &
      ImageNet-O, iNaturalist, OpenImage-O, Texture &
      BiT-S, DeiT,  RepVGG, ResNet-50, ResNet-50-D, Swin-T, VIT-B-16 \\
    \rowcolor[HTML]{FED8E5} 
    KLM; MLS \cite{hendrycks2019scaling} & ImageNet-21K; ImageNet-1K, Places & Species (categories); BDD-Anomaly, StreetHazards (segmentation)
      & Mixer-B-16; ResNet-50, TResNet-M, ViTB-16 \\
    \rowcolor[HTML]{FED8E5} 
    REACT \cite{sun2021react} &
      ImageNet-1K &
      iNaturalist, Places, SUN, Textures &
      MobileNet, ResNet \\
    % \rowcolor[HTML]{FED8E5} 
    % MLS &
    %   ImageNet-21K-P, ImageNet-1K, Places, PASCAL VOC, MS-COCO &
    %   Categories from the Species dataset, 20   out-of-distribution classes from  ImageNet-21K. These classes have no overlap with ImageNet-1K, PASCAL VOC, or MS-COCO &
    %   ResNet, ViT, MLP mixer \\
    \rowcolor[HTML]{FED8E5} 
    GRAM \cite{huang2021importance}&
      ImageNet-1K &
      iNaturalist, SUN, Places, Textures &
      DenseNet-121, ResNetv2-101 \\
    \rowcolor[HTML]{F3D5B0} 
    RMDS \cite{ren2021simple} &
       CIFAR-10, CIFAR-100 &
      CIFAR-10,   CIFAR-100 &
      BiT, CLIP, VIT-B-16 \\
    \rowcolor[HTML]{CFE7FF} 
    EBO \cite{liu2020energy} &
      CIFAR-10 &
      ISUN, Places, Texture, SVHN, LSUN &
      WideResNet \\
    \rowcolor[HTML]{F3D5B1} 
    MDS \cite{lee2018simple} &
      CIFAR-10 &
      SVHN, TinyImageNet, LSUN, Adversarial Examples &
      DenseNet, ResNet \\
    \rowcolor[HTML]{FED8E5} 
    ODIN  \cite{liang2017enhancing} &
      CIFAR-10 &
      LSUN, SVHN, TinyImageNet &
      DenseNet, ResNet \\
    \rowcolor[HTML]{FED8E5} 
    MSP \cite{hendrycks2016baseline} &
      CIFAR-10 &
      SUN (Gaussian) &
      WideResNet 40-4 \\ 
    \hline
    \multicolumn{4}{c}{OOD Detectors for Adversarial Robustness} \\ \hline    
    \rowcolor[HTML]{70AD47} 
    ALOE \cite{chen2020robust} &
      CIFAR-10, CIFAR-100, GSTRB &
      PGD attack &
      DenseNet \\
    \rowcolor[HTML]{70AD47} 
    OSAD \cite{shao2020open}  &
      CIFAR-10, SVHN, TinyImageNet &
      FGSM, PGD attack &
      ResNet-18 \\
    \rowcolor[HTML]{70AD47} 
    ADT \cite{azizmalayeri2022your} &
      CIFAR-10, CIFAR-100 &
      FGSM, PGD attack &
      ViT \\
    \rowcolor[HTML]{70AD47} 
    ATOM \cite{chen2021atom} &
       CIFAR-10, CIFAR-100, SVHN &
      PGD attack &
      WideResNet \\
    % \rowcolor[HTML]{70AD47} 
    % HAT \cite{rade2021reducing} &
    %    CIFAR-10, CIFAR-100, SVHN &
    %   PGD attack&
    %   WideResNet \\
    \rowcolor[HTML]{FED8E5} 
    SAFE \cite{wilson2023safe} &
      PASCAL-VOC, DeepDrive &
      FGSM attack &
      RegNetX4.0, ResNet-50 \\
    \hline \bottomrule[1pt]
\end{tabular}
}
\end{table*}
